# Supplementary material for: Adaptive Super-Resolution Imaging Without Prior Knowledge Using a Programmable Spatial-Mode Sorter
Source: arXiv:2409.04323 source file (2024-12-12)
Supplement: Supplementary file 1 [file Supplamentary_Material.tex]

\documentclass[9pt]{osa-supplemental-document}
\setboolean{shortarticle}{false}
\usepackage{placeins} % Required for \FloatBarrier

\title{Supplementary Material}
\author{} %leave this blank
%% DO NOT ADD AUTHOR INFORMATION HERE; IT WILL BE ADDED DURING PRODUCTION

\begin{document}

\section{Cross-talk}
To obtain the best experimental results the matrix we tried to optimize is cross-talk. We define cross-talk as follows:
 \begin{equation}
    C=\frac{I_{\rm{absent}}}{I_{\rm{absent}}+I_{\rm{present}}}
 \end{equation}
where $I_{\rm{present}}$ is the intensity found in the expected output location on the detector when the input is a pure mode, and $I_{\rm{absent}}$ is the intensity found in all the other spots.

To characterize our system properly we first found the cross-talk matrices when sorting in the Hadamard basis. The reason we chose to characterize our system with that basis is that creating pure Hadamard code words can be easily done with the SLM. The following tables show the cross-talk when sorting two and four Hadamard modes respectively:

\begin{figure}[ht]
\centering
\fbox{\includegraphics[width=\linewidth]{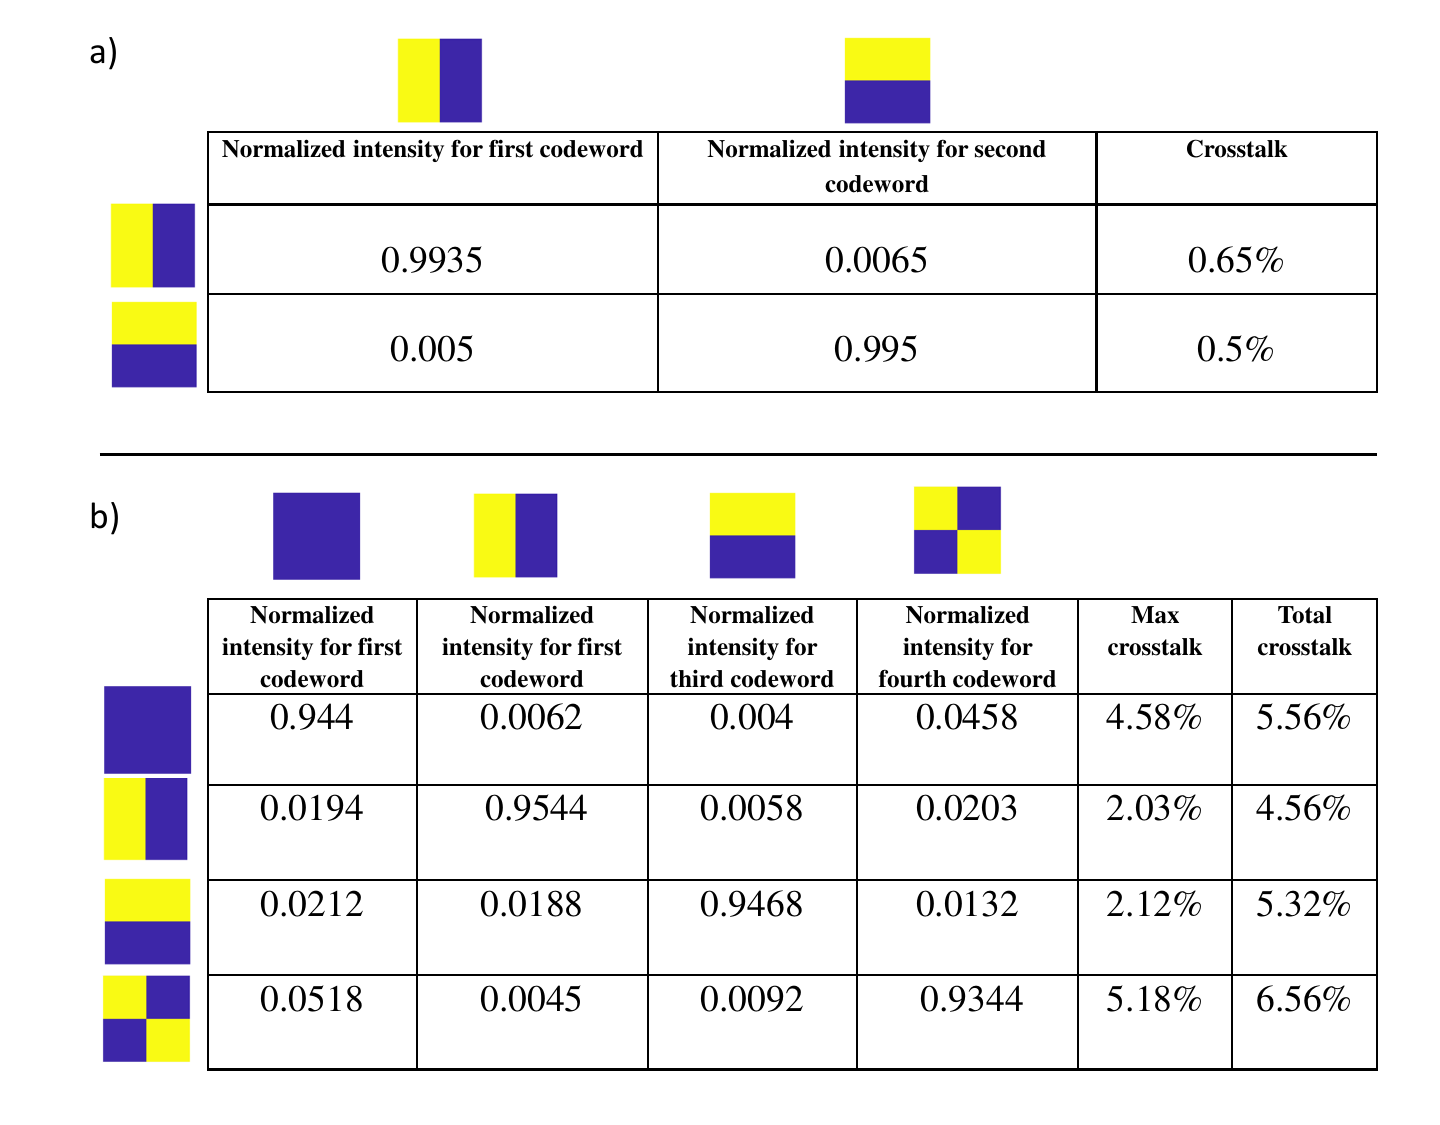}}
\caption{a) Cross-talk matrix when sorting 2 modes from Hadamard basis. b) Cross-talk matrix when sorting 4 modes from Hadamard basis.}
\label{fig:Crosstalk_hadamard}
\end{figure}

\section{Aberration Correction}
The liquid crystal array of our SLM (Holoeye PLUTO-2.1-VIS-016) is on a substrate that is not perfectly flat. This will cause aberrations in the system if not accounted for. To account for this, the aberrations were measured using a Twyman-Green interferometer, and a phase mask, which was calculated using the 4-measurements method which can be found in \cite{Creath1988} was displayed on the whole SLM to cancel these aberrations. The results of the aberration correction phase mask can be seen in Fig. \ref{fig:aberration}.

 \begin{figure}[htbp]
\centering
\fbox{\includegraphics[width=\linewidth]{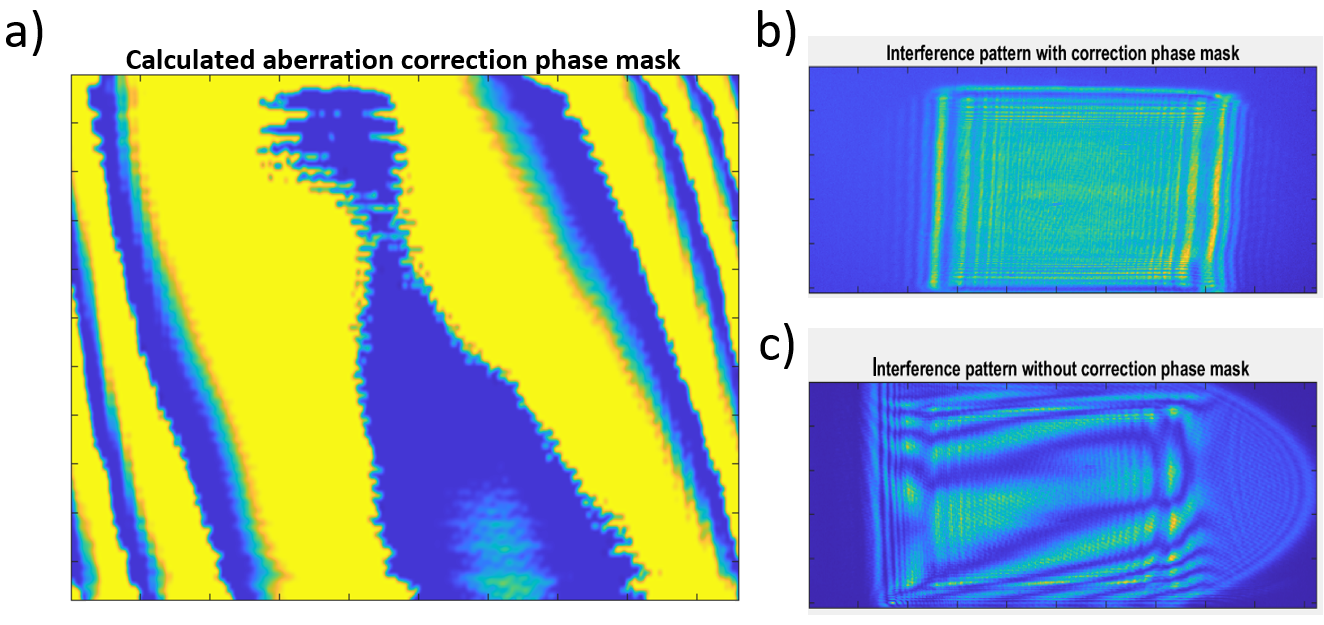}}
\caption{a) The applied phase mask used to correct for aberrations due to the SLM. b) The interferogram between a flat mirror and the SLM with the aberration correction phase mask. c) The interferogram between a flat mirror and the SLM without the aberration correction phase mask. }
\label{fig:aberration}
\end{figure}

\section{Loss in the system}
In our system, most of the loss comes from the SLM. All other sources of loss are negligible. There are 3 main factors that contribute to the loss from the SLM:

1. Grating efficiency: In our system, the SLM is tilted downwards and each phase mask on the SLM is displayed on top of a blazed grating (which, theoretically, sends 100\% of the light to the first diffraction order), such that the first diffraction order travels through the system while the zeroth diffraction order is reflected down. By designing our system in such a way we ensure that 100\% of the light that travels through the system is phase-modulated, as all the un-modulated light is reflected down and out of the system. The efficiency of a blazed grating when applied on the SLM is 82\%.

2. Reflectivity: the reflectivity of the SLM is  65\%. 

3. Fill factor: the fill factor of the SLM due to pixelation is 75\%.

Overall, we have 3 bounces off the SLM after we encode the object. Therefore, the loss from the SLM can be described as follows:
\begin{equation}
    \rm{Loss}=1-(0.82\times0.65\times0.75)^3=0.9361\approx94\%
\end{equation}
Note that the total measured loss in the system was found to be closer to 98\%. This additional loss is most likely coming from not directing all the light perfectly to its designated spots, so some of the light lands in different locations on the detector that are not measured.

There are other sources of loss in the system that are related to the detector and therefore are not added to the calculation above of excess loss due to mode sorting. According to the iXon Ultra 897 hardware guide, the quantum efficiency of the detector is assumed to be 90\%. Ths means that there will be another 10\% loss of the light hitting the detector both when using direct imaging and mode sorting.
\section{Power calibration and camera characterization}
In our experiment we operated in the low photon flux regime. Therefore, we used our Andor iXon 897 EMCCD in its photon counting mode. To do that we cooled the detector to $-80$ degrees Celsius using the EMCCD's internal cooling mechanism.
The first thing that we did was to characterize the dark counts on the detector and compare it to the expected shot noise, as shown in Fig.\ref{fig:Shot Noise}.
\begin{figure}[ht]
\centering
\fbox{\includegraphics[width=\linewidth]{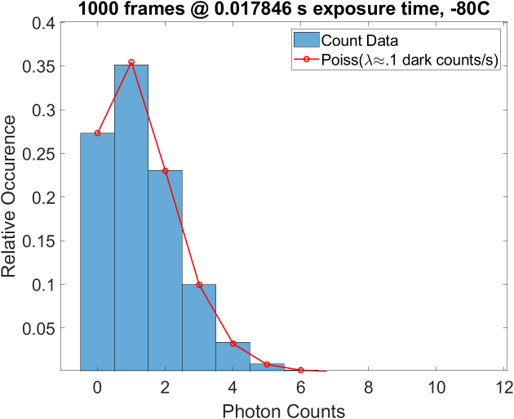}}
\caption{Histogram: Experimental results for number of photons counted on each pixel during 1000 frames. Red line: Expected results for the number of photons counted on each pixel during 1000 frames using the poison noise formula where the mean number of occurrences in the interval is 0.1.}
\label{fig:Shot Noise}
\end{figure}

When calibrating the power we aim for a 1\% probability of multi-photon events occurring in the brightest pixel in each frame. This probability can be mathematically described as follows:
\begin{equation}
    P_0(\lambda)+P_1(\lambda)=e^{-\lambda}{+}\lambda e^{-\lambda}=0.99 ,
\end{equation}
where $\lambda$ is the mean number of occurrences in an interval. 
When solving the equation above we find that the value that we want is $\lambda=0.1486 \frac{\rm{Photons}}{\rm{Pixel/}\rm{Frame}}$, and therefore when plugging in the found value to the equation above we find that through 1000 frames with the proper illumination, and with the absence of noise we want to see 138 \textit{clicks} in the brightest pixels. We noted that with just noise we got around 12 \textit{clicks} in the brightest pixel. Therefore, when calibrating the power we aimed to get 150 \textit{clicks} on the brightest pixel. 

\section{Compensation for noise and dark clicks}
To compensate for the dark clicks and noise that were detected we took the following steps:

1. For the centroid estimation, since we supposedly do not know where the signal should exist, we created a threshold such that only pixels with a number of photons that is larger than a third of the number of photons on the brightest pixel are taken into account. 

2. For both the direct imaging and sorting, we counted the average number of clicks on pixels which we supposed to be completely dark and subtracted the average background noise from the whole image (without allowing a pixel to have a negative photon count).

3. Cropping the direct images around the signal to minimize the contribution of the remaining background to the likelihood calculation.

4. Optimizing the size of the spot from which we count photons when mode sorting. The larger the spot is the more photons that can contribute to the likelihood calculation, but, some of these additional photons come from noise.

\section{Estimator Bias}
Another way in which we could quantify our system's performance and compare it to our simulation is by looking at the variance and the bias of our estimators separately. Rather than comparing the exact values, it is important to notice the trends and how they compare. {Note that the plots in this section should be interpreted the same way as Fig. 8 in the main text.}

{In Fig. \ref{fig:Centroid_bias} one can see the Box Whisker plot for our experimental centroid estimation. From this plot it is apparent that as the separation increases, the variance of our measurement increases, however, we see no bias in the data, as the mean and the median stay around 0.}

In Fig. \ref{fig:DirectBias_exp} one can see the box-whisker plot of our experimental data and in Fig. \ref{fig:DirectBias_sim} one can see the Box-Whisker plot of our Monte-Carlo simulation. In both plots, we can see a similar trend and notice that we do not have almost any bias at any separation and that as the separation increases the variance decreases. This is to be expected since direct imaging performs at its best when the separation between point sources is 1 Rayleigh unit or more.

\begin{figure}[ht]
\centering
\fbox{\includegraphics[width=\linewidth]{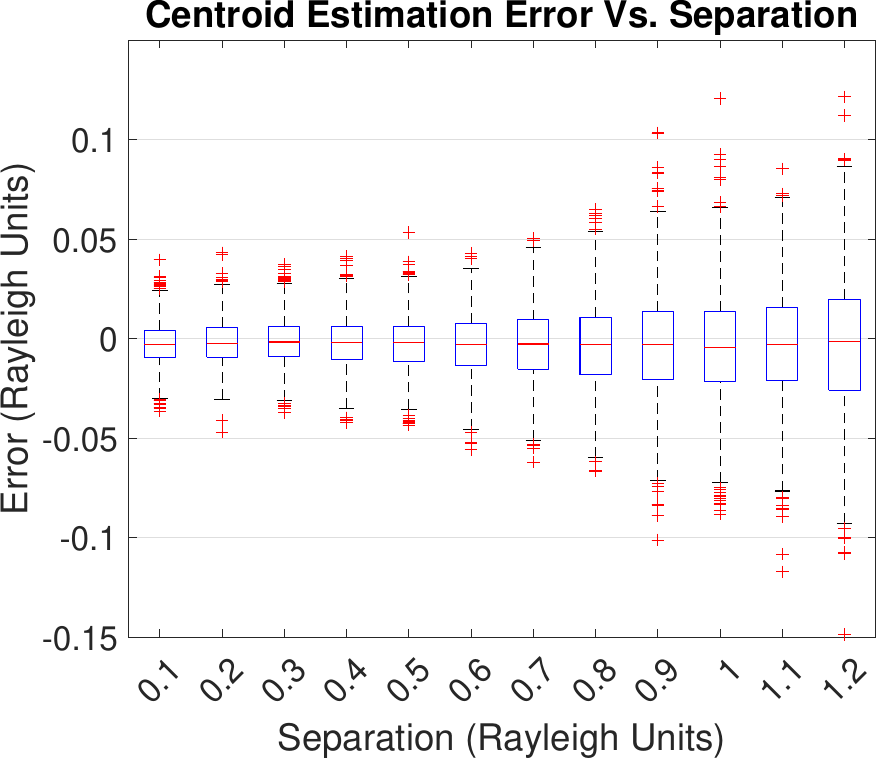}}
\caption{Centroid estimation experimental bias.}
\label{fig:Centroid_bias}
\end{figure}

\begin{figure}[ht]
\centering
\fbox{\includegraphics[width=\linewidth]{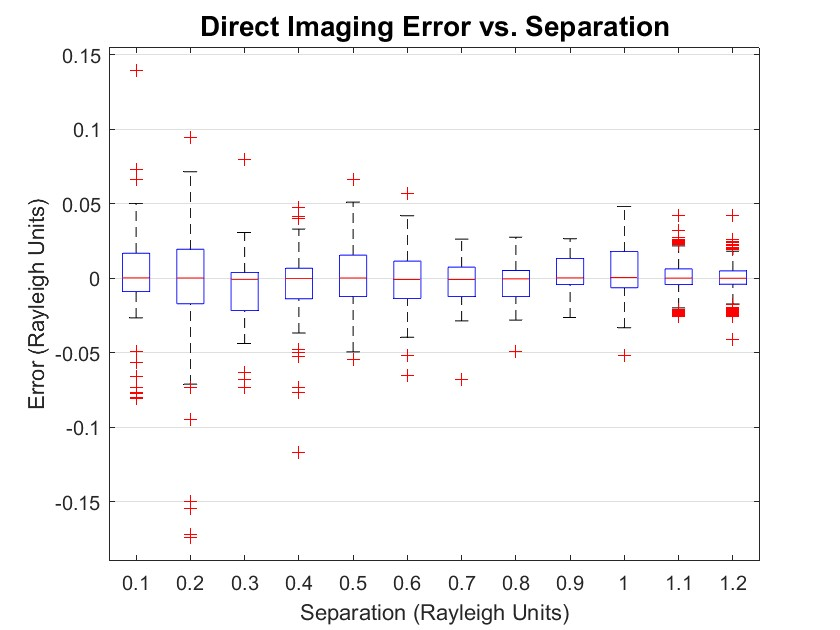}}
\caption{Direct Bias Experimental.}
\label{fig:DirectBias_exp}
\end{figure}

\begin{figure}[ht]
\centering
\fbox{\includegraphics[width=\linewidth]{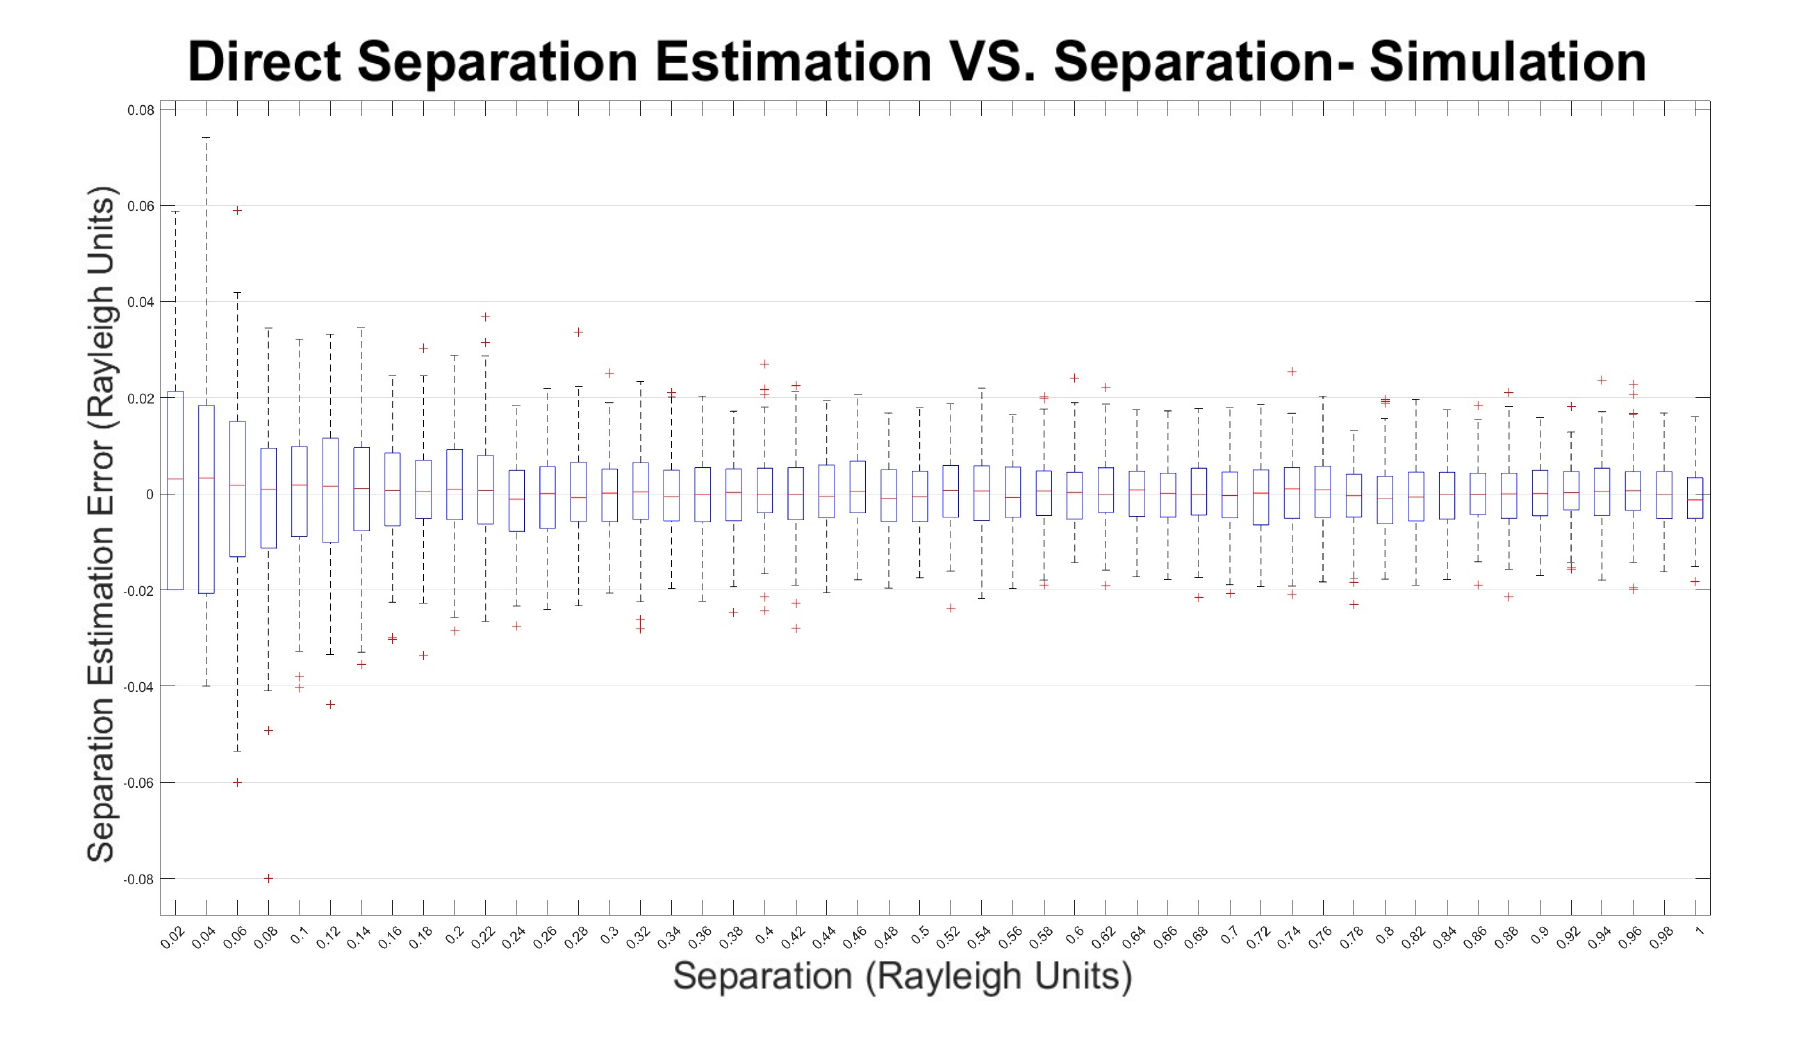}}
\caption{Direct Bias Simulation.}
\label{fig:DirectBias_sim}
\end{figure}

Fig. \ref{fig:SortingBias_sim} shows the box-whisker plot of our mode sorter in a Monte Carlo simulation. The main noticeable trends are that as the separation between the point sources increases, the variance also increases and that we do not see almost any bias at any separation. The same trend can be seen in Fig. \ref{fig:SortingBiasLookup_exp} which shows the box-whisker plot of our experimental mode sorter when processing the data in the comparison to characterization method. When looking at Fig. \ref{fig:SortingBiasLikelihood_exp}, which shows the box-whisker plot of our experimental mode sorter when estimating the separation using a maximum likelihood estimator we do see some bias that increases as the separation gets farther from 0.2 Rayleigh units. However, we do see a smaller variance when comparing it to  Fig. \ref{fig:SortingBiasLookup_exp}. This leads us to believe that there was a slight misalignment in our system that translated into a bias in our data. These results are still encouraging as it is obvious that with a correction to the bias, our mode sorter performs even better than can be seen in Fig. 7a and therefore further enhances the performance in the deep sub-Rayleigh regime.

\begin{figure}[ht]
\centering
\fbox{\includegraphics[width=\linewidth]{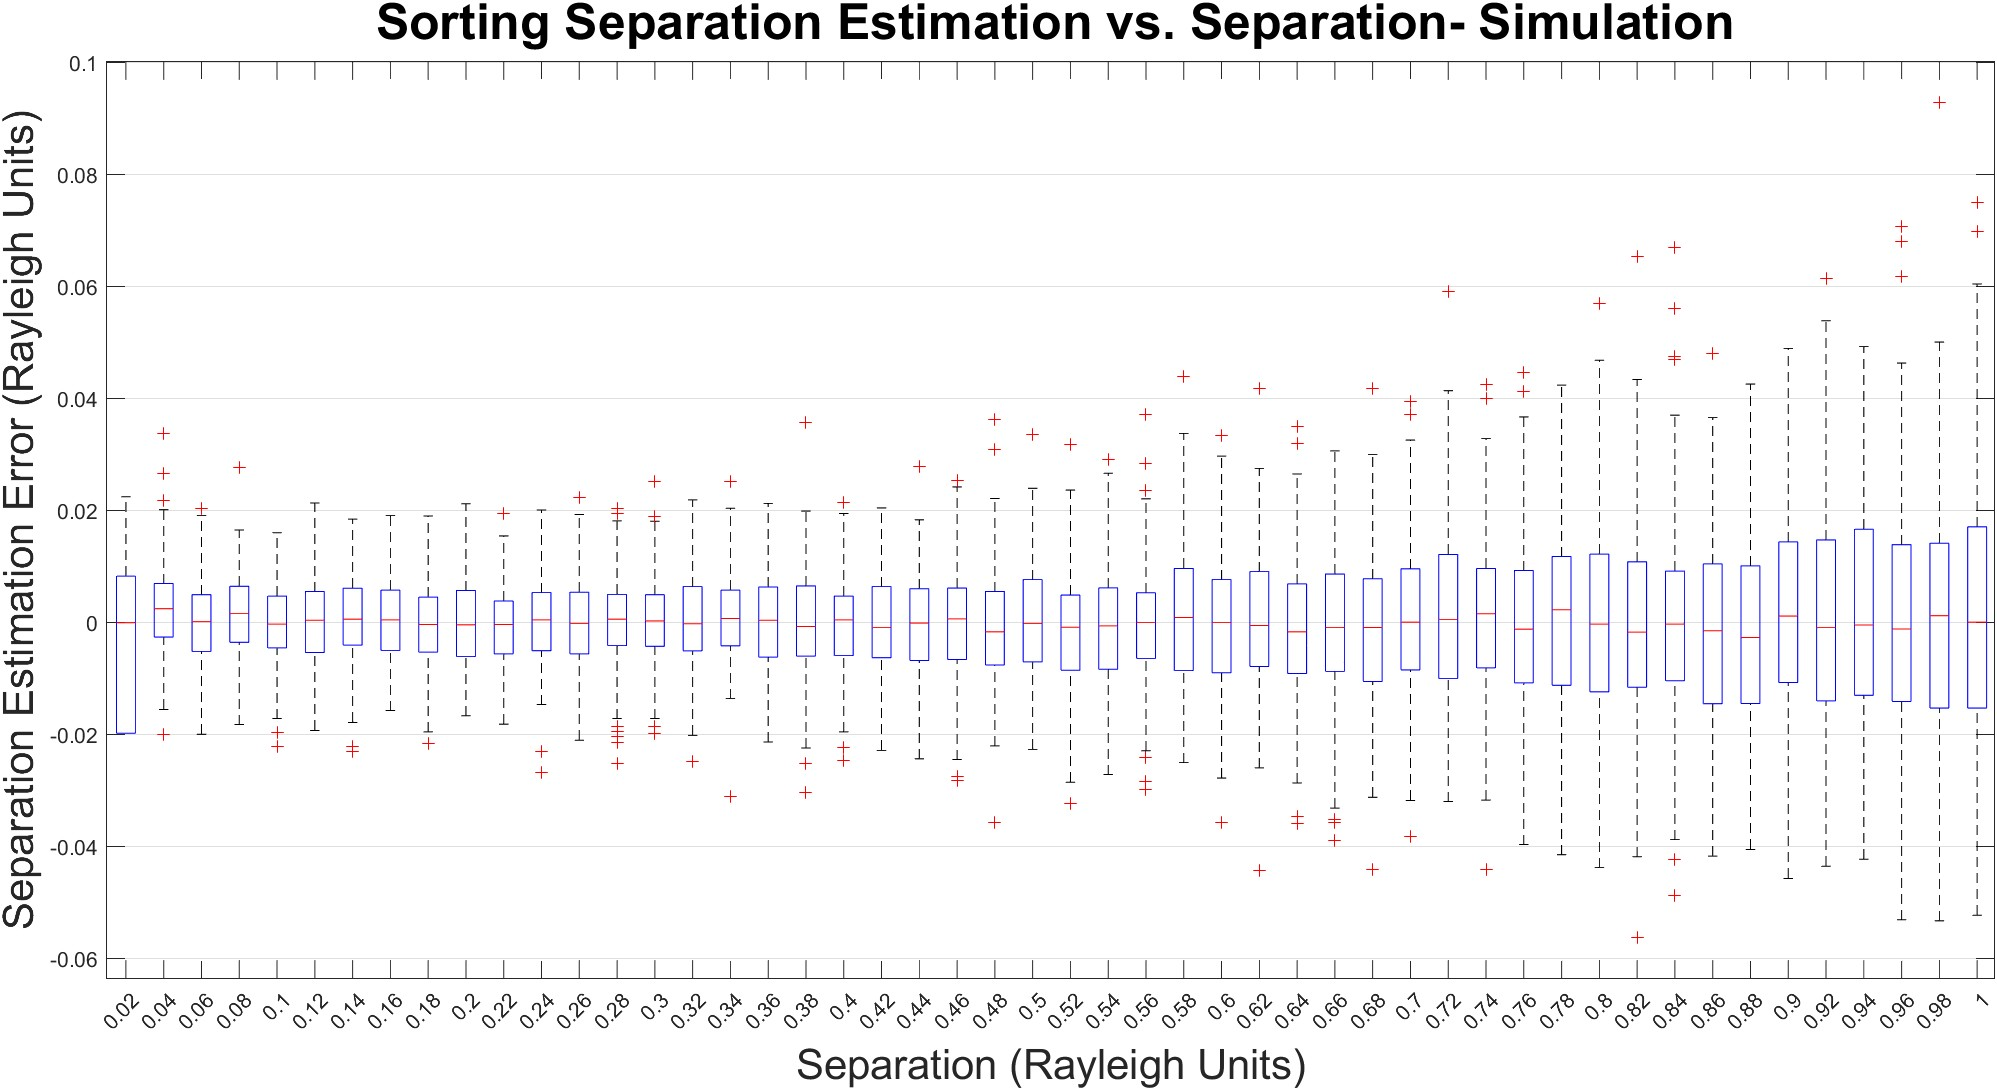}}
\caption{Sorting Bias simulation.}
\label{fig:SortingBias_sim}
\end{figure}

\begin{figure}[ht]
\centering
\fbox{\includegraphics[width=\linewidth]{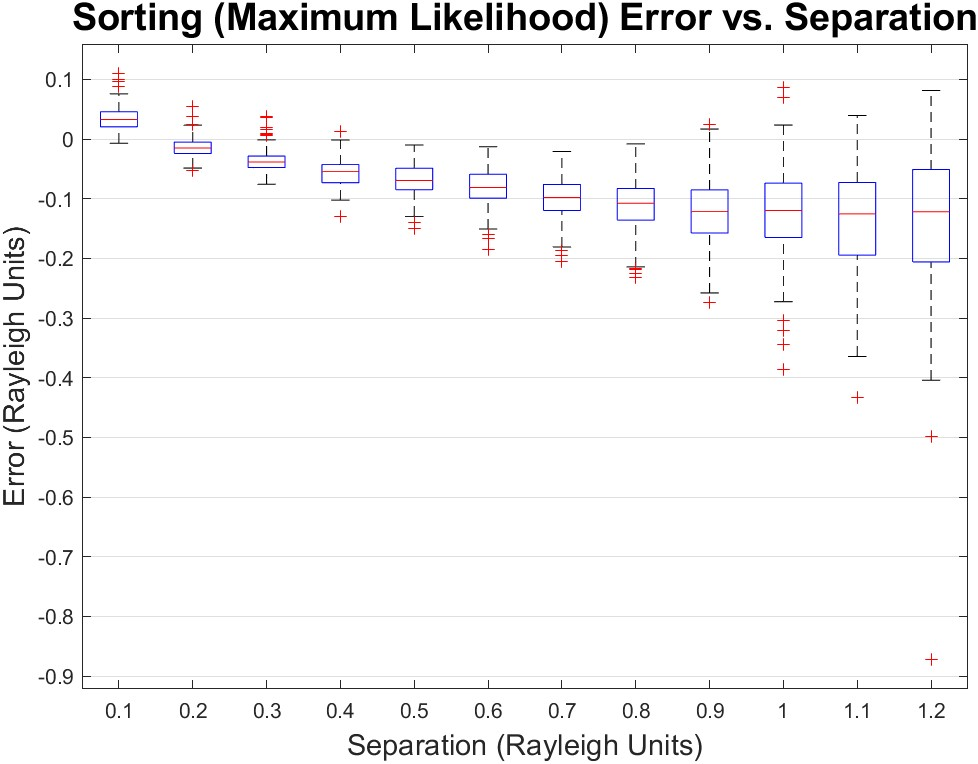}}
\caption{Sorting (Likelihood) Bias Experimental.}
\label{fig:SortingBiasLikelihood_exp}
\end{figure}

\begin{figure}[ht]
\centering
\fbox{\includegraphics[width=\linewidth]{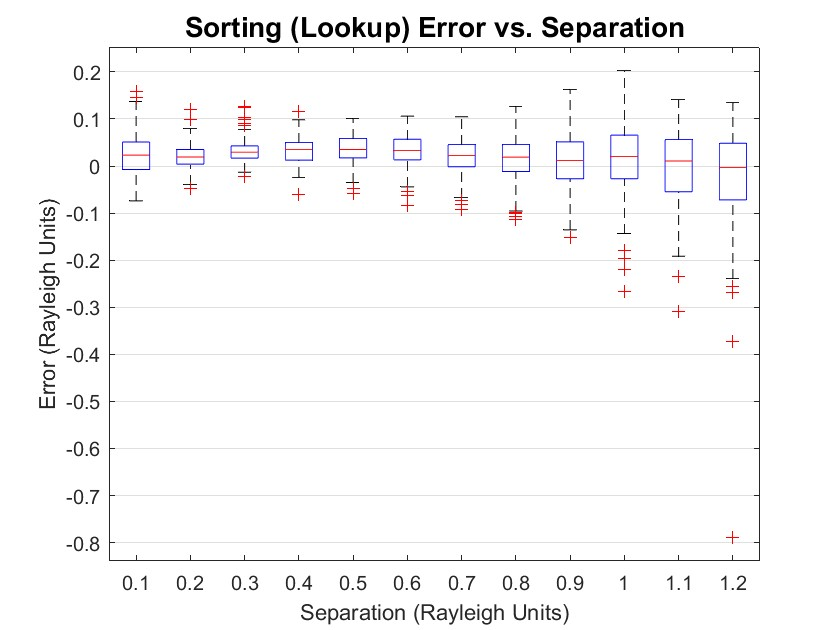}}
\caption{Sorting (Comparison to characterization) Bias Experimental.}
\label{fig:SortingBiasLookup_exp}
\end{figure}
\FloatBarrier
\bibliography{Bibliography}

\end{document}
